# Supplementary material for: Partial Mobilization: Tracking Multilingual Information Flows Amongst Russian Media Outlets and Telegram
Source: arXiv:2301.10856 source file (2025-03-08)
Supplement: Supplementary file 1 [file appendix.tex]

\section{Appendix}
\begin{table}[htb]
\centering
\scriptsize
\begin{tabular}{lr}
Top Twitter & \# Russian  \\ 
 Accounts & Websites    \\ \midrule
{DmytroKuleba} & 8 \\
{trussliz} & 7  \\
DefenceHQ & 7 \\
{SecBlinken}  & 7\\
{ZelenskyyUa}  & 7 \\
{Bundeskanzler}  & 7 \\
JosepBorrellF  & 7  \\
vonderleyen  & 6\\
{eucopresident}   & 6  \\
{TokayevKZ} & 6  \\
\end{tabular}
 \caption{\label{tab:top-youtube}Top Twitter accounts mentioned by our set of 17 Russian Websites. }  
\end{table}
\begin{table}[htb]
\centering
\scriptsize
\begin{tabular}{lr}
Top YouTube & \# Telegram  \\ 
 Channels & Channels    \\ \midrule
\foreignlanguage{russian}{Россия 24} & 61 \\
\foreignlanguage{russian}{Анатолий Шарий} & 50  \\
Max Chronicler & 46 \\
\foreignlanguage{russian}{Комсомольская Правда }  & 39\\
\foreignlanguage{russian}{Информационное агентство БелТА}  & 39 \\
\foreignlanguage{russian}{RT на русском}  & 34 \\
Metametrica  & 34  \\
Fox News  & 32\\
\foreignlanguage{russian}{ИЗОЛЕНТА live}   & 31  \\
\foreignlanguage{russian}{Телеканал Рада} & 31  \\
\end{tabular}
 \caption{\label{tab:top-youtube}Top YouTube channels mentioned by our set of 732 Telegram Channels. }  
\end{table}
\clearpage
